# Supplementary material for: Geometric Numerical Integration of the Assignment Flow
Source: arXiv:1810.06970 source file (2018-10-05)
Supplement: Supplementary file 1 [file Appendix.tex]

% !TEX root =  ../ExponentialIntegrators.tex

\section{Proof of Lemma \ref{lem:dS}}

The proof follows after two preparatory Lemmata.
